# Supplementary material for: Physically Real-time Infrared Attack against Optical Flow Estimation Networks
Source: arXiv:2607.26651 source file (2026-07-29)
Supplement: Supplementary file 1 [file X_suppl.tex]

\clearpage
\setcounter{page}{1}
\maketitlesupplementary

\section{Experimental Setup}

In our experiments, the hyper-parameters were set as follows: \(\alpha = 0.9\), \(\beta = 0.1\), the default camera distance was 80 cm, the default ambient light level was 0.5, the default moving speed was 18 cm/s, and the number of layers in the default AGN network was set to 8.

\section{Weighted Factors in Eq. \ref{eq:fitness}}
To determine the optimal values of \(\alpha\) and \(\beta\), we conducted a series of experiments with multiple values. Given that \(\alpha\) and \(\beta\) are two independent factors, we constrained their sum to 1 (\(\alpha + \beta = 1\)) to reduce the number of experiments. We varied \(\alpha\) from 0 to 1, and the corresponding \(\beta\) was automatically determined as \(1 - \alpha\). The experimental results are illustrated in Fig. \ref{fig:supp_1}.

\begin{figure}[ht]
\centering
\includegraphics[width=0.4\textwidth]{graph/supp_1.pdf}
\caption{The performance of RILA in different weighted factors.} 
\label{fig:supp_1}
\end{figure}
From the above figure, we could notice thar with $\alpha$ increasing, the AIV is increasing steadily and AIP is not stable. RILA performed best when $\alpha=0.9$.
